# Supplementary material for: Symmetry Perception by Deep Networks: Inadequacy of Feed-Forward Architectures and Improvements with Recurrent Connections
Source: arXiv:2112.04162 source file (2022-01-22)
Supplement: Supplementary file 1 [file appendix.tex]

\section{Additional RSA Figures}

We generated additional violin plots in \ref{fig:rsa_violins_1},\ref{fig:rsa_violins_2},\ref{fig:rsa_violins_3},\ref{fig:rsa_violins_4},\ref{fig:rsa_violins_5}, f{fig:rsa_violins_6} in order to more clearly see the distrobution of homogeneity across different features. These were generated by subdividing each model's dissimilarity scores into categories according to the two images compared. For example, a dissimilarity score in "band" is between two images with the same band property, either both having a band or both not having a band. All dissimilarity scores between non-matching images in a particular grouping were assigned to the "AC" (across) group.

\begin{table}[t!]
\begin{center}
\begin{tabular}{c|c|c}
    \textbf{model} &  \textbf{layer} & \textbf{units} \\
    \hline
    % Darius' data
    % SQN       & relu\_conv1  & 784 \\
    % AlexNet   & fc7   &  4096 \\
    % GoogleNet   & inception\_5b-output,   & 50176 \\
    % IRN        & conv\_7b\_ac   & 98304 \\
    % IV3        & mixed10   & 131072 \\
    % RN18      & res5b-relu   & 25088 \\
    % LSTM      & final cell & 25600 \\
    % Transformer & ?? & 512 \\

    % TODO: get names and activation sizes for Shobhita's data. Not sure if info above is still accurate.
    InceptionResNetV2       & INSERT_LAYER_NAME  & INSERT_ACTIVATION_SIZE \\
    InceptionV3   & INSERT_LAYER_NAME   &  INSERT_ACTIVATION_SIZE \\
    ResNet101   & INSERT_LAYER_NAME,   & INSERT_ACTIVATION_SIZE \\
    Xception        & INSERT_LAYER_NAME   & INSERT_ACTIVATION_SIZE \\
    DenseNet        & INSERT_LAYER_NAME   & INSERT_ACTIVATION_SIZE \\
    Dilated      & INSERT_LAYER_NAME   & INSERT_ACTIVATION_SIZE \\
    Transformer & INSERT_LAYER_NAME & INSERT_ACTIVATION_SIZE \\
    LSTM3      & INSERT_LAYER_NAME & INSERT_ACTIVATION_SIZE \\

\end{tabular}
    \caption{Table of each model architecture which was included in the RSA analysis along with the name of the layer which the activations were recorded from and the number of units in that layer.}
\end{center}
\end{table}
    \begin{figure}
        \includegraphics[width=\linewidth]{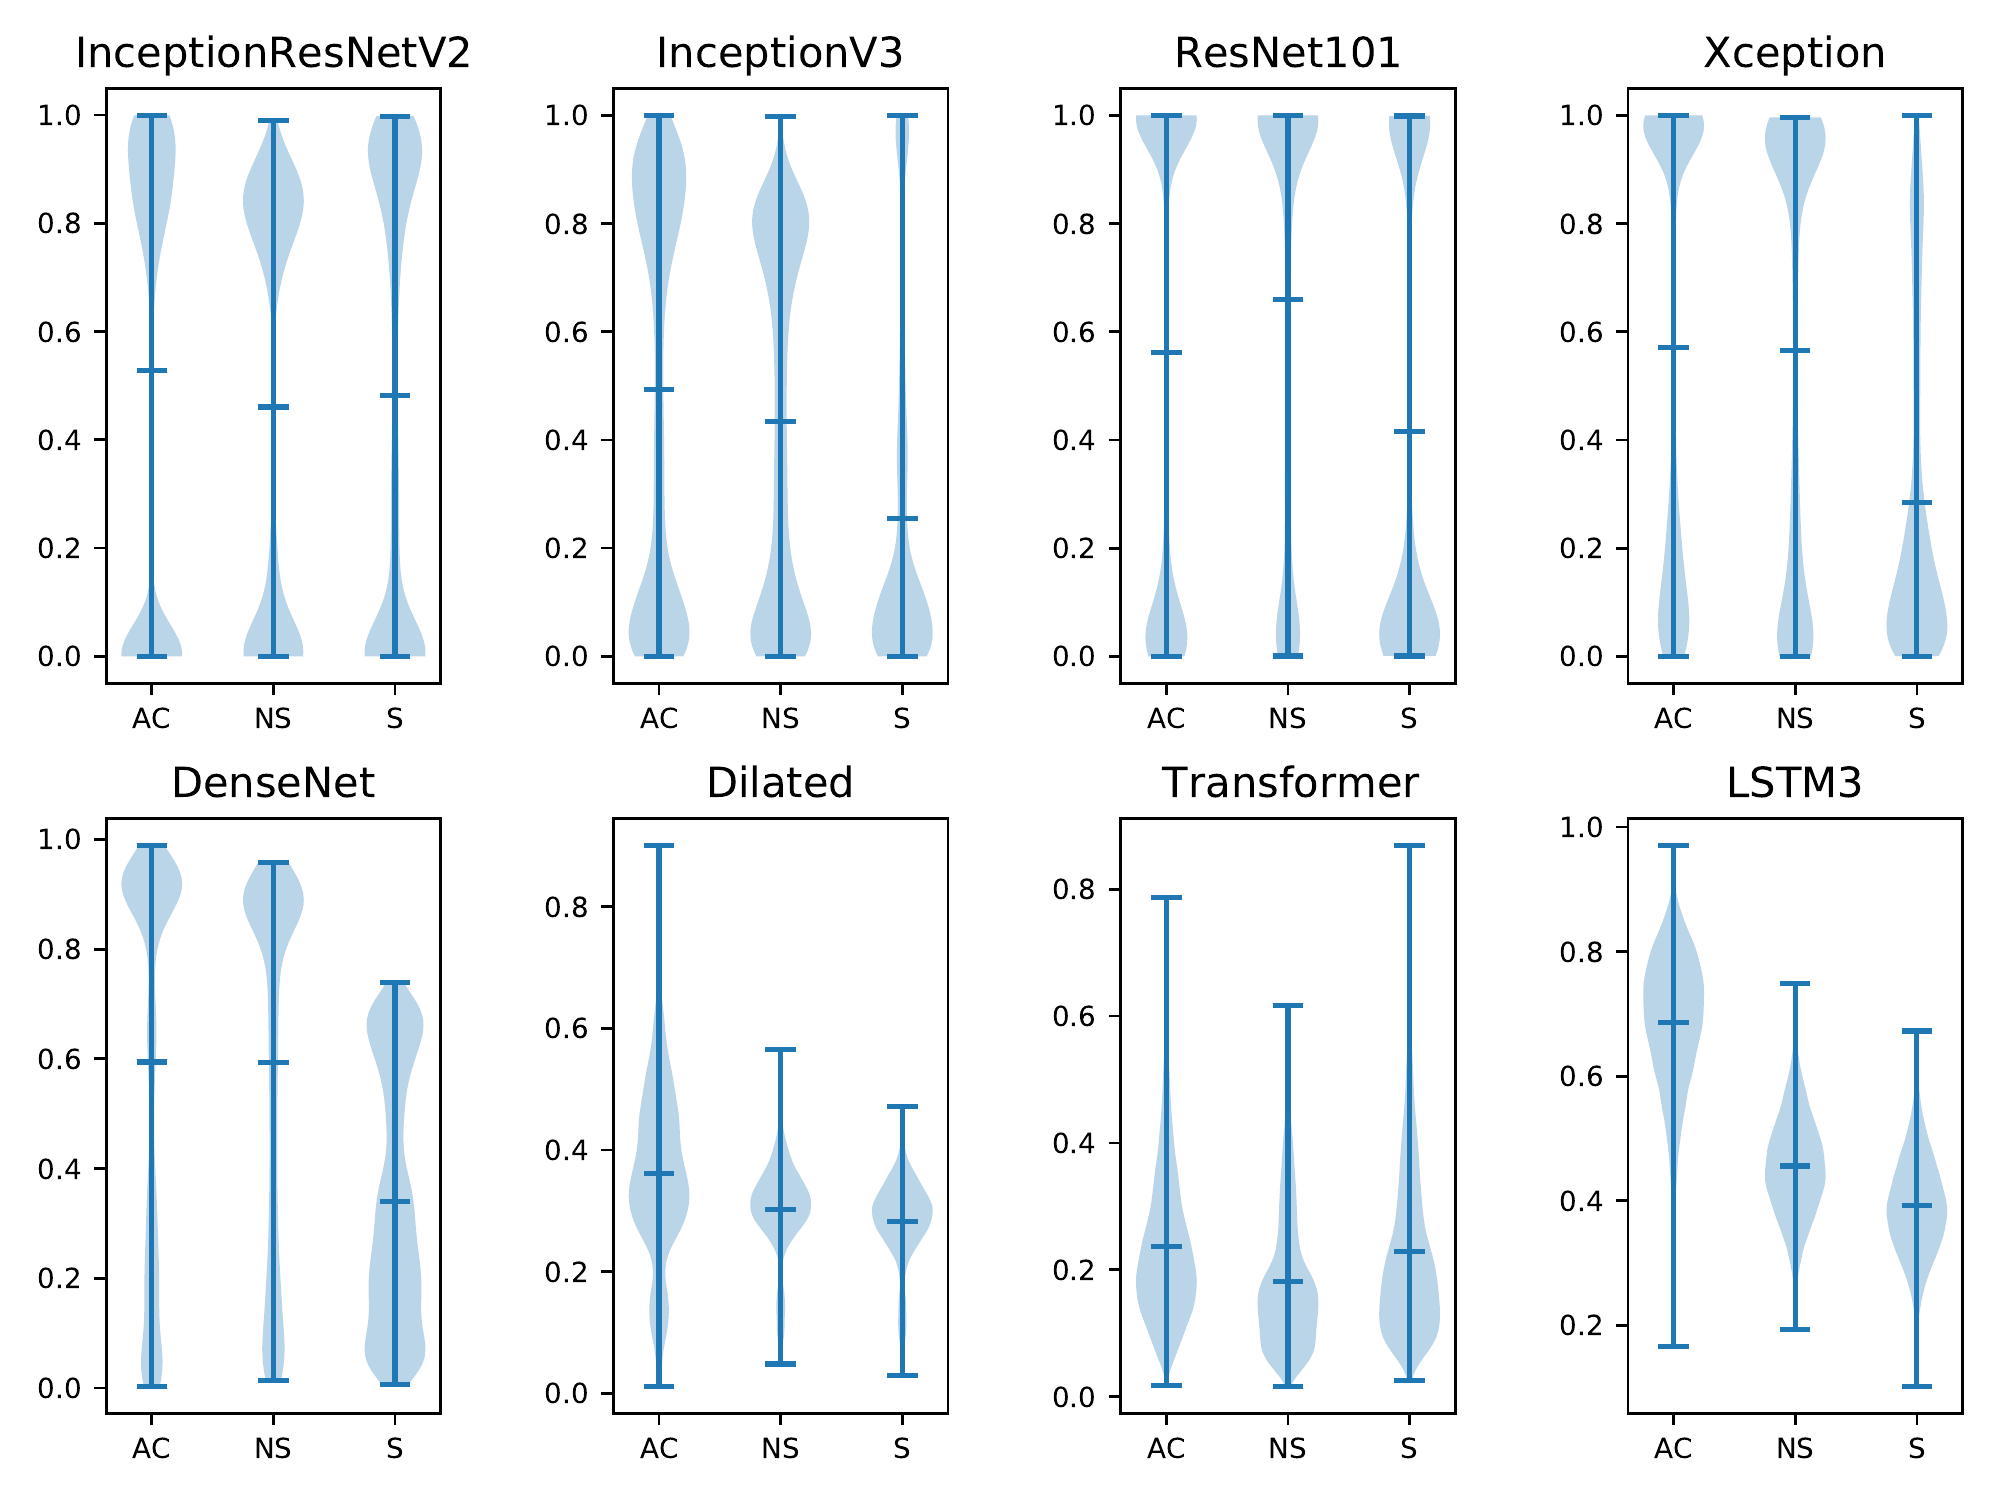}
        \caption{Another representation of the L2 norm output in which each violin represents the dissimilarity in a particular grouping. "AC" stands for across, and is the dissimilarity across features (such as between asymmetric and symmetric images).}
        \label{fig:rsa_violins_1}
    \end{figure}
    
        \begin{figure}
        \includegraphics[width=\linewidth]{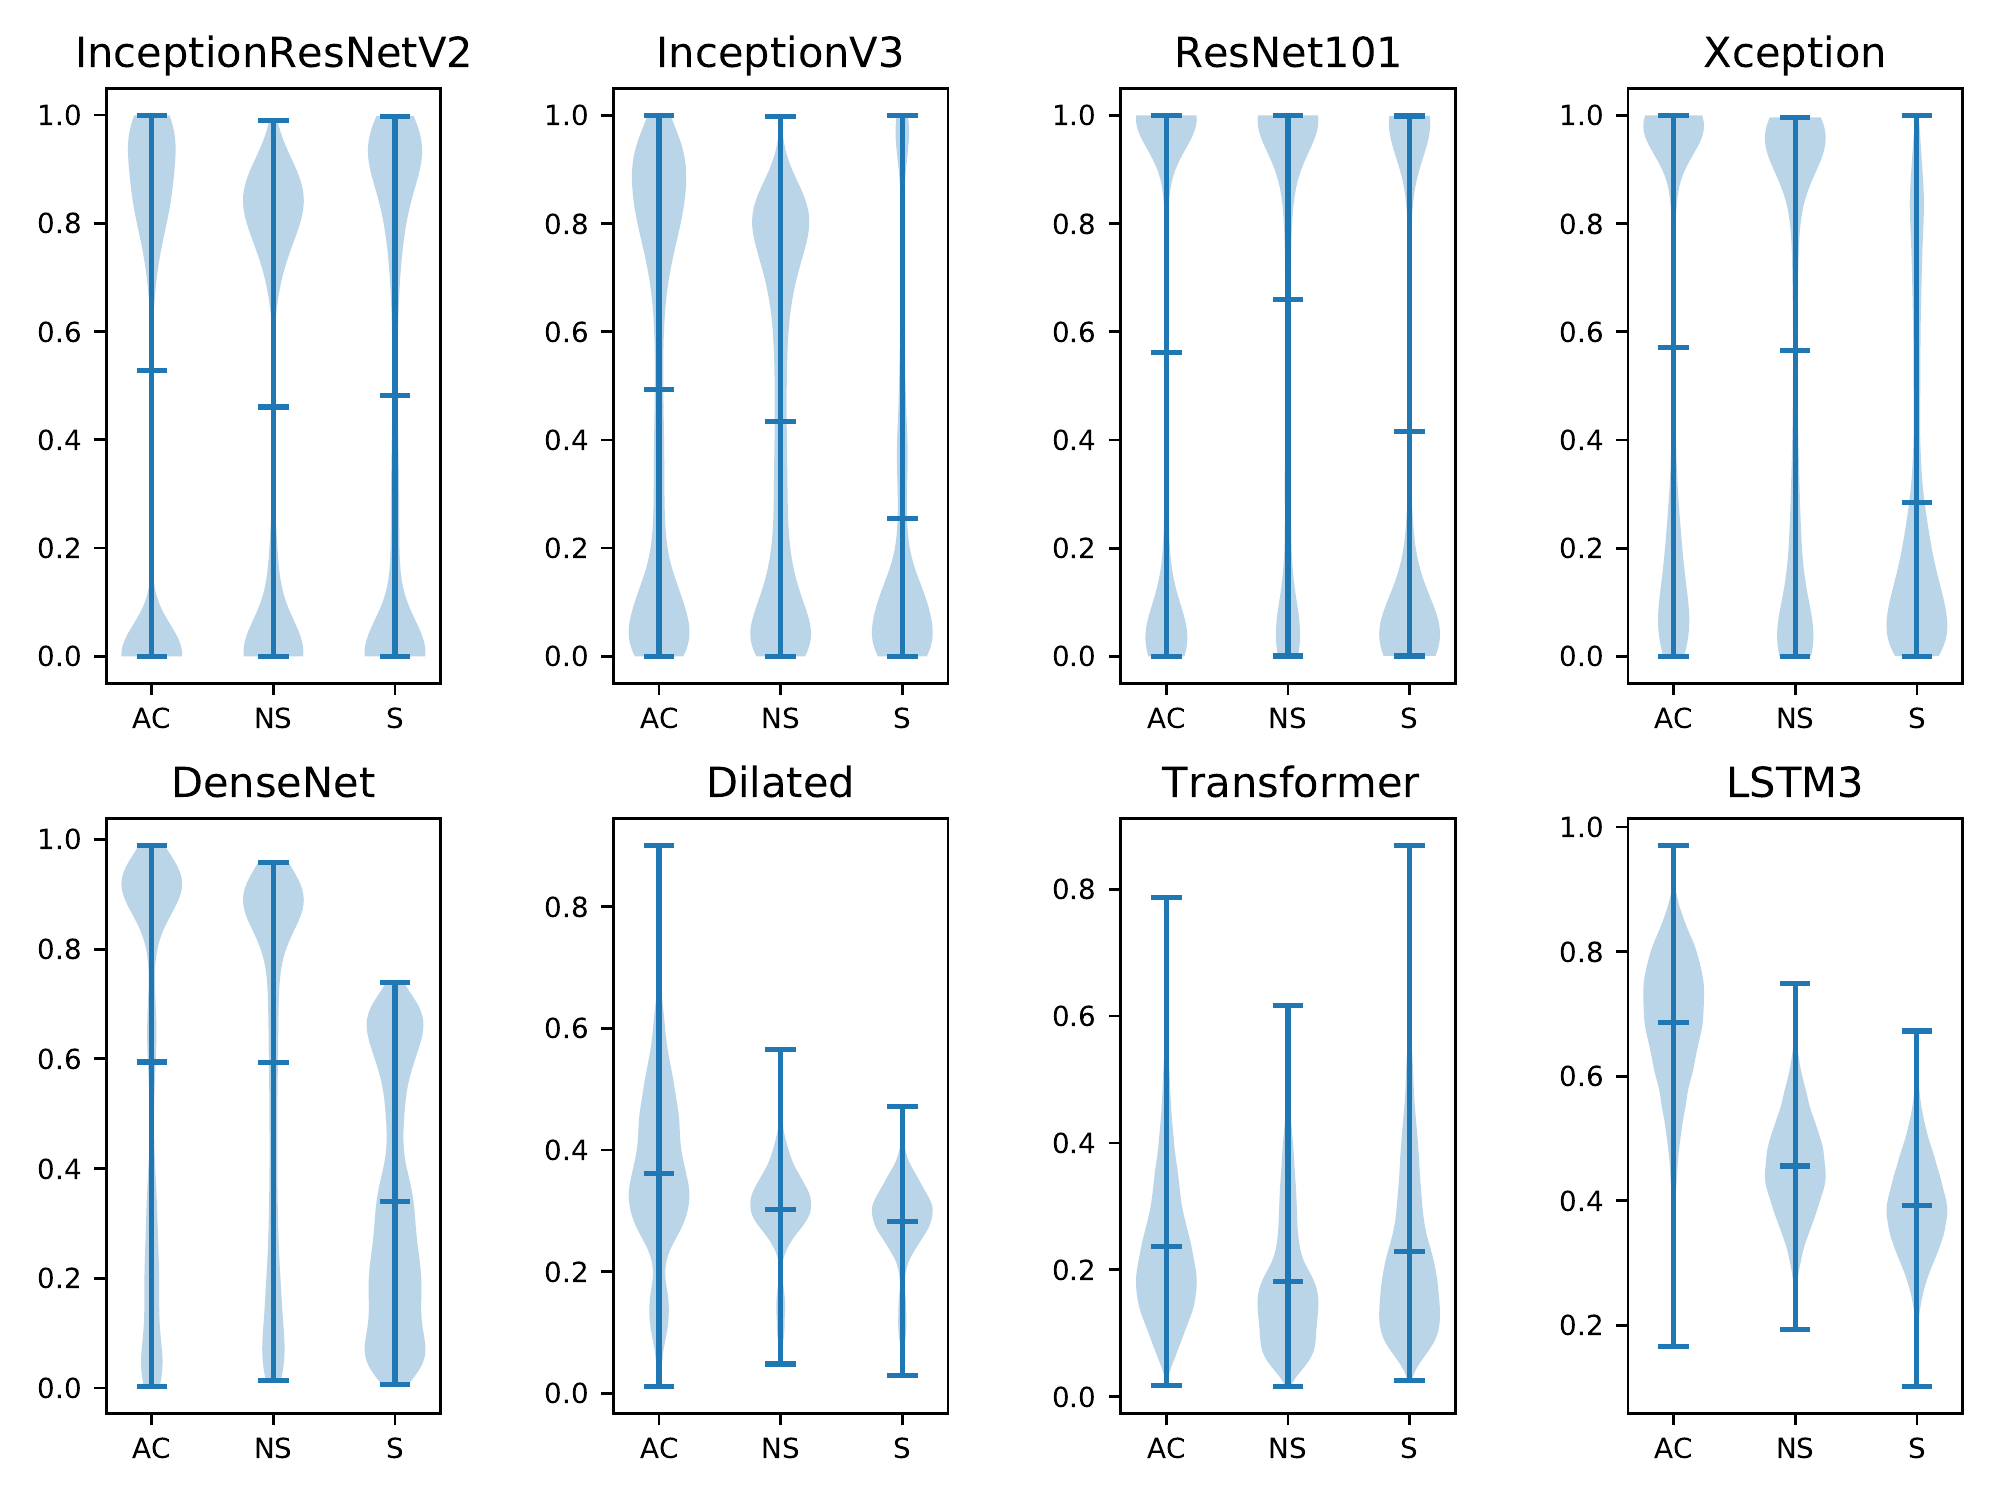}
        % \caption{Another representation of the L2 norm output in which each violin represents the dissimilarity in a particular grouping. "AC" stands for across, and is the dissimilarity across features (such as between asymmetric and symmetric images).}
        \label{fig:rsa_violins_2}
    \end{figure}
    
    \begin{figure}
        \includegraphics[width=\linewidth]{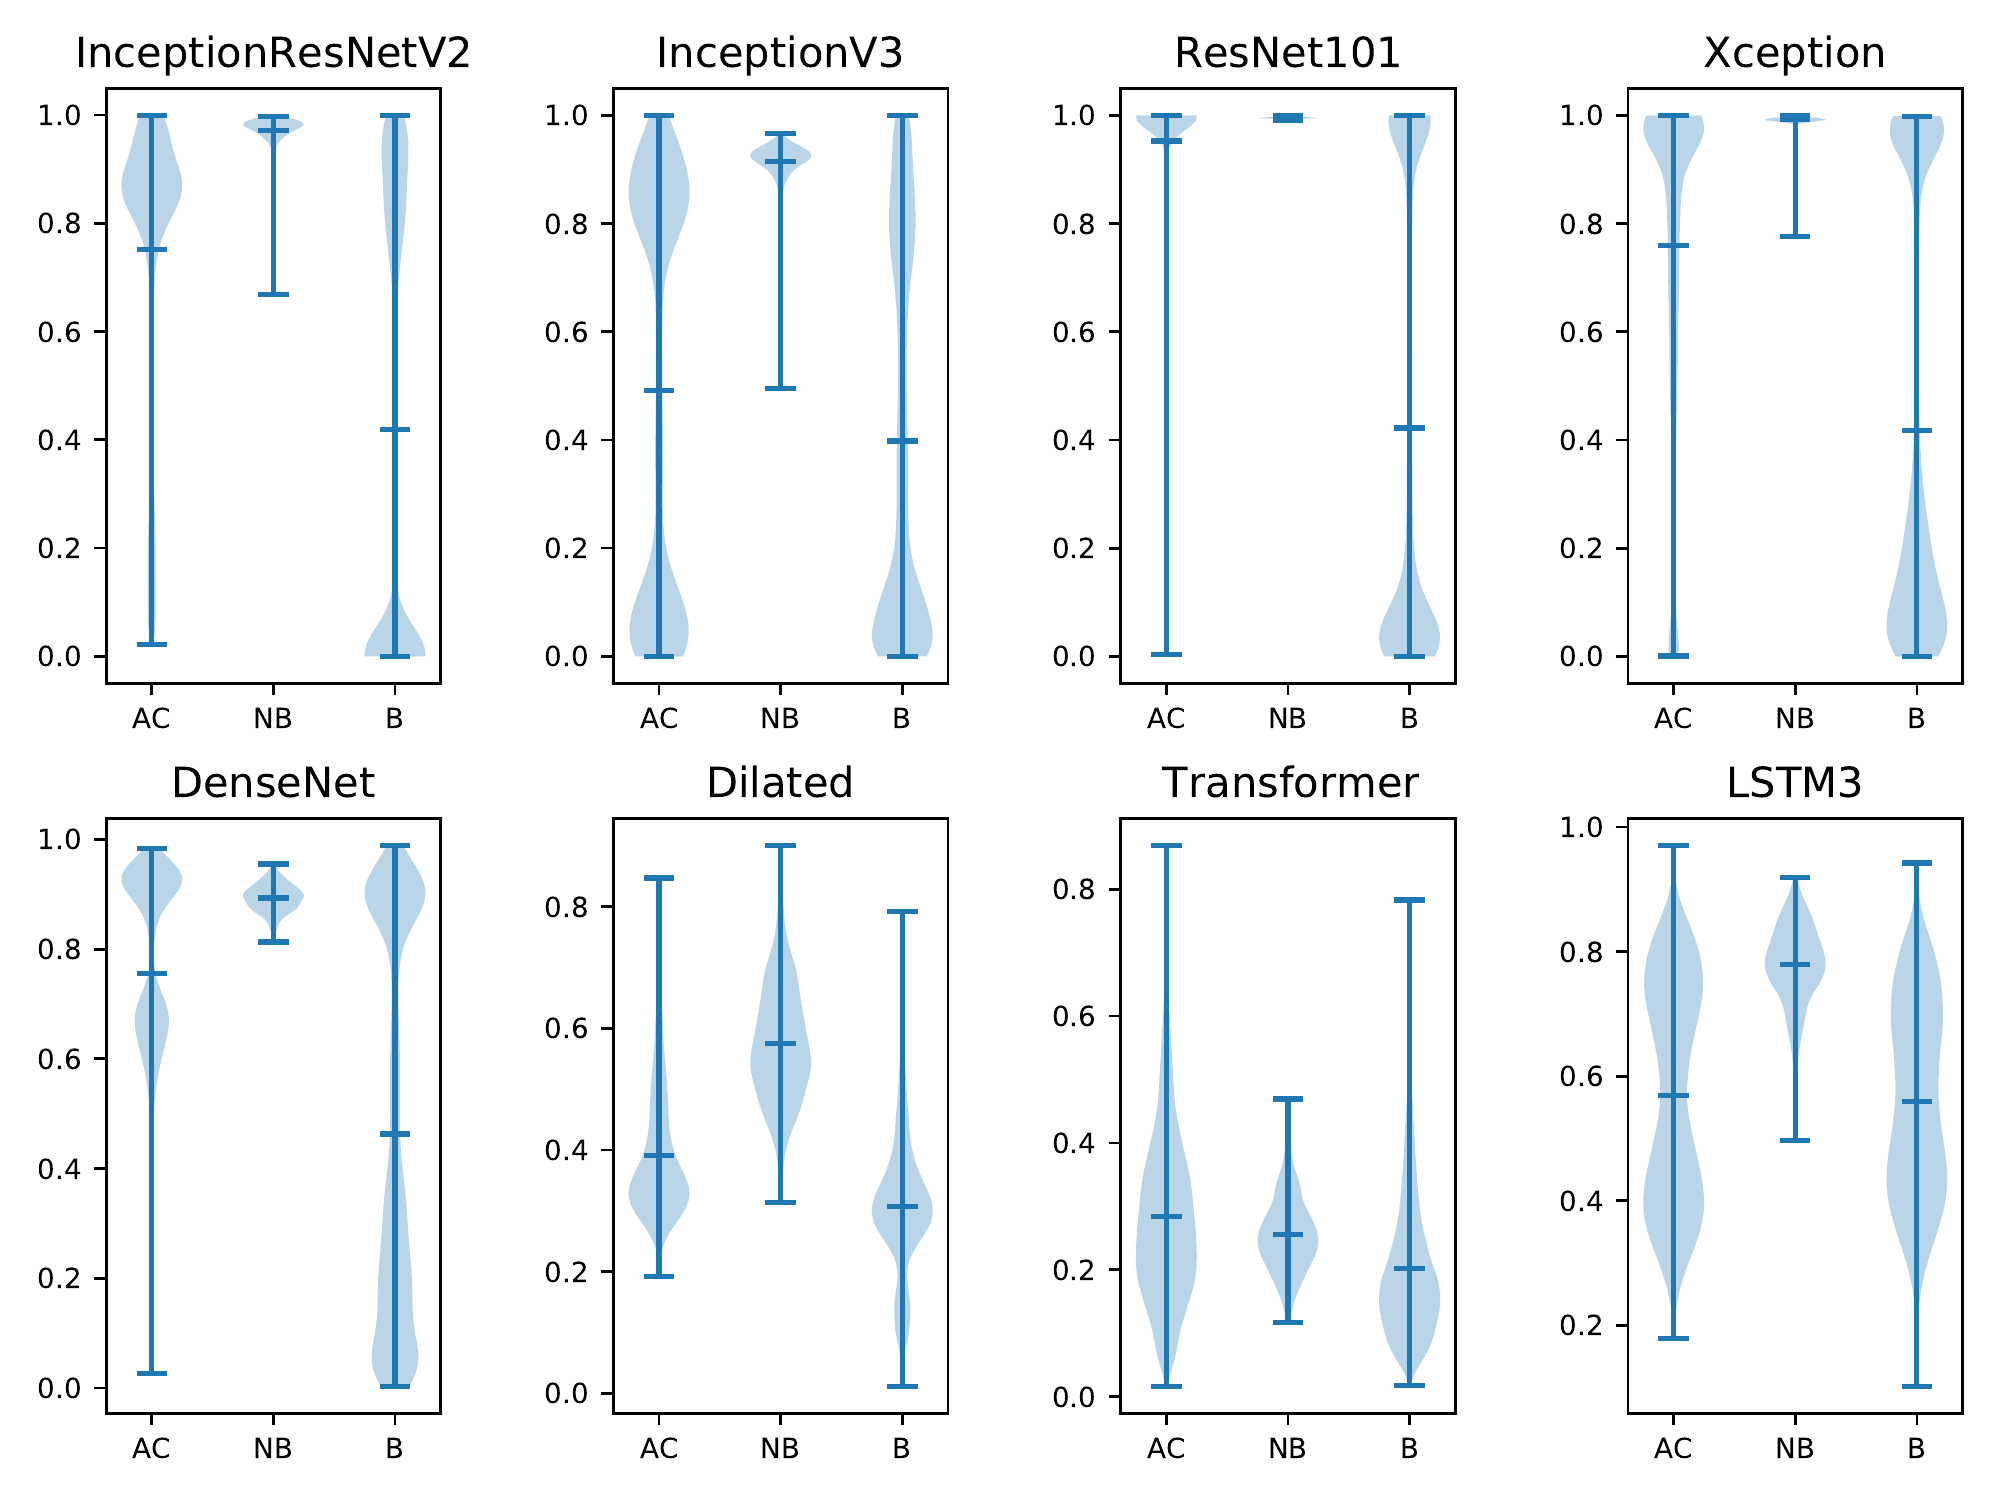}
            % \caption{Another representation of the L2 norm output in which each violin represents the dissimilarity in a particular grouping. "AC" stands for across, and is the dissimilarity across features (such as between asymmetric and symmetric images).}
     \label{fig:rsa_violins_3}
    \end{figure}
    
     \begin{figure}
        \includegraphics[width=\linewidth]{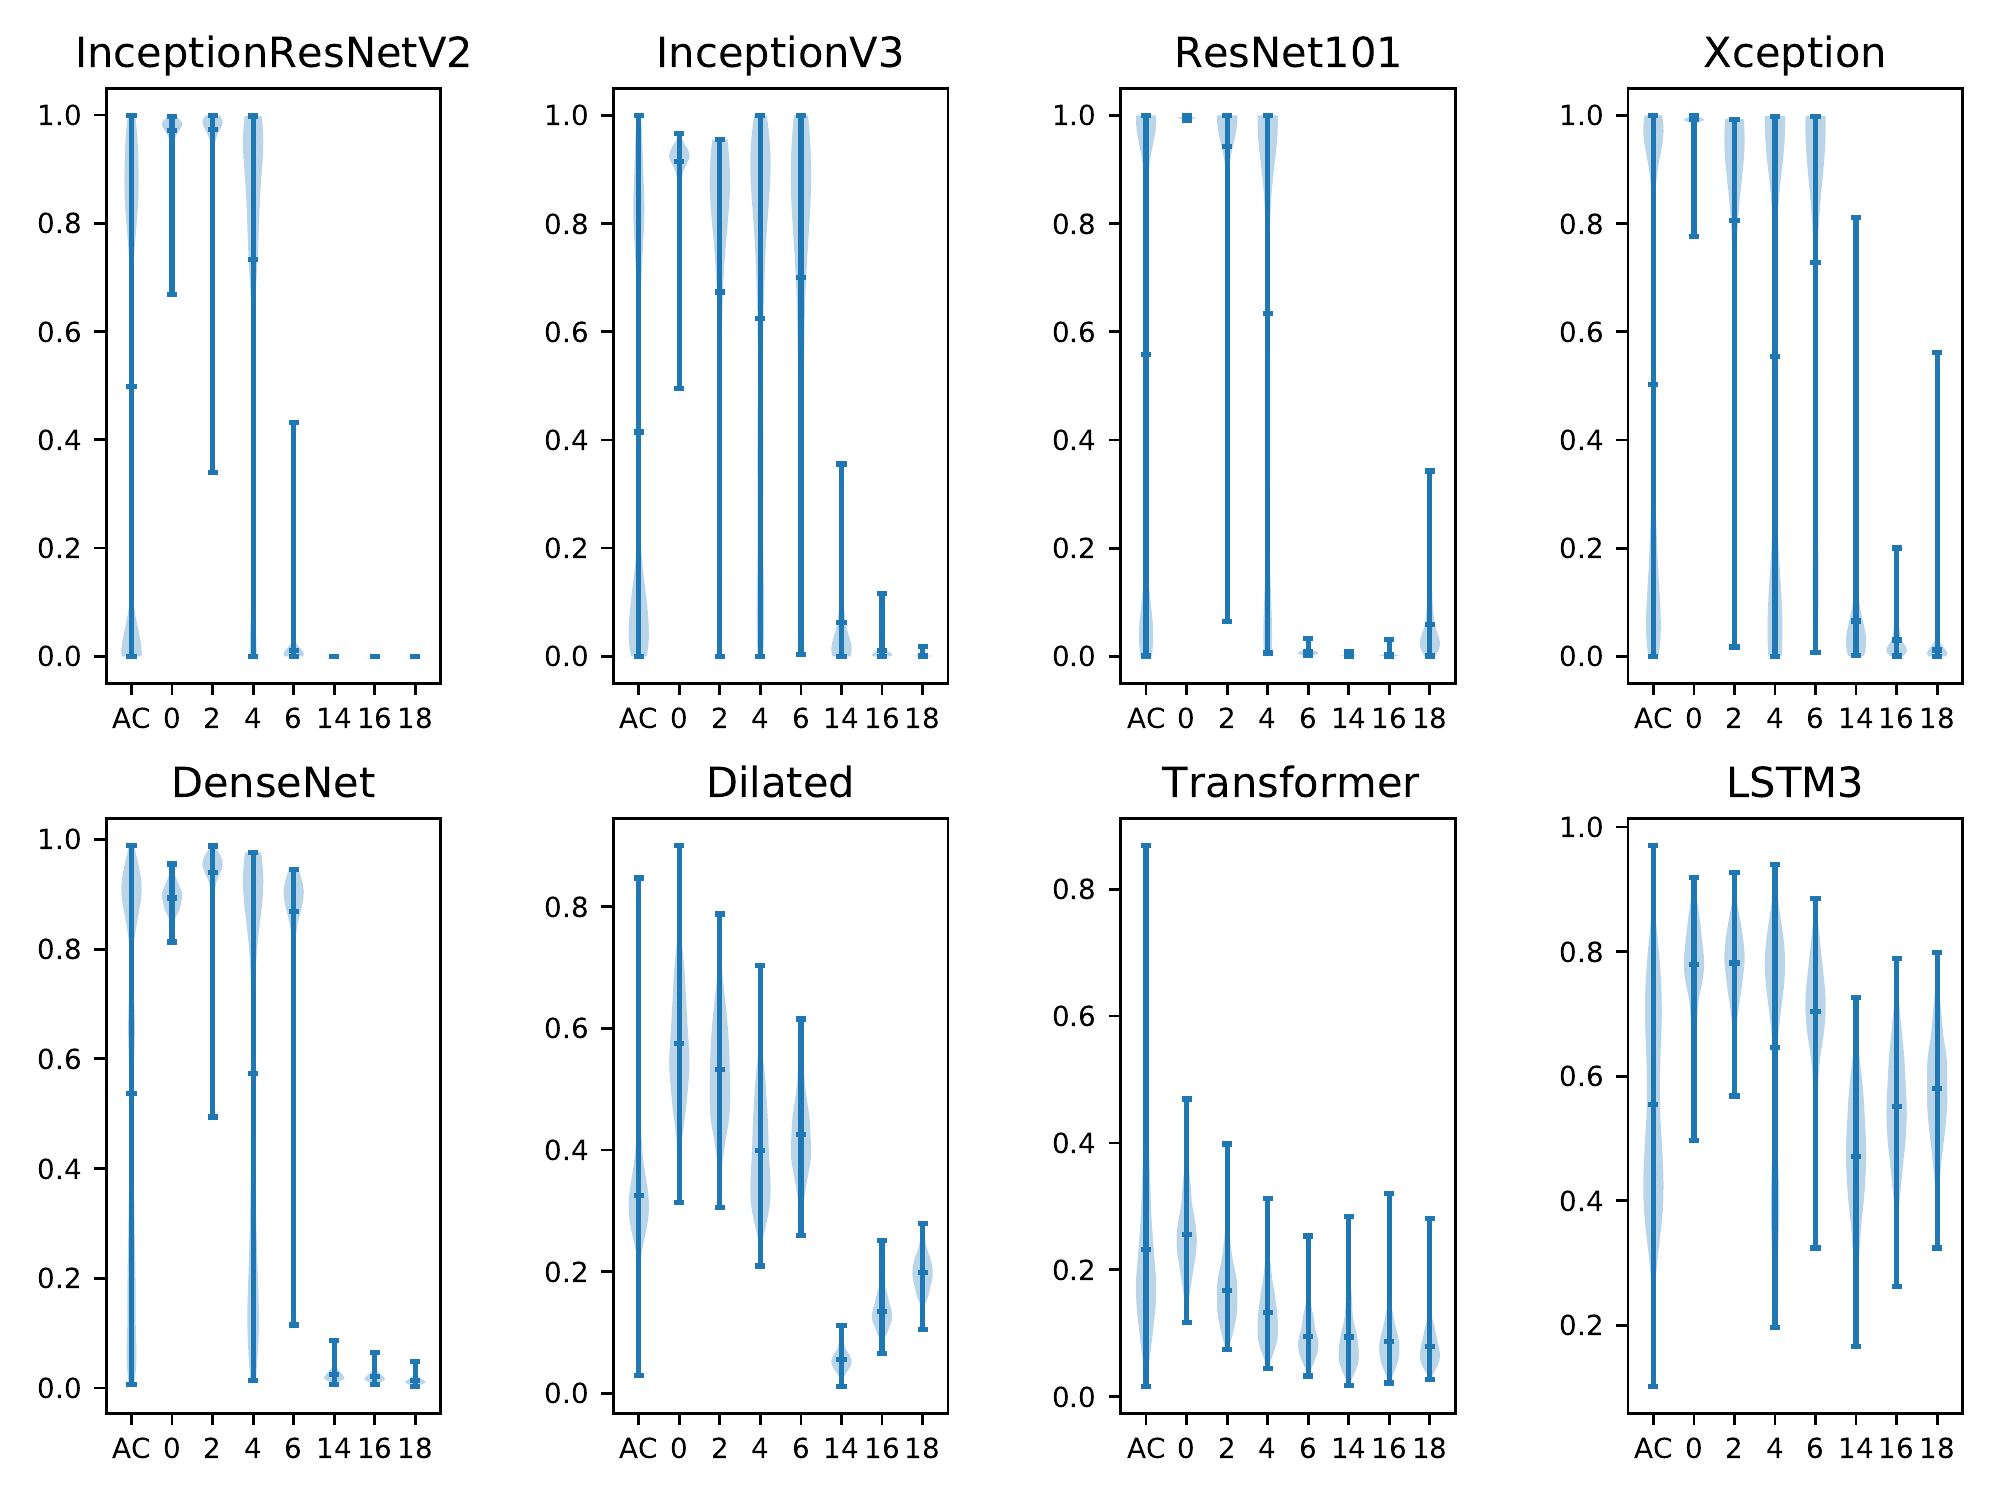}
                % \caption{Another representation of the L2 norm output in which each violin represents the dissimilarity in a particular grouping. "AC" stands for across, and is the dissimilarity across features (such as between asymmetric and symmetric images).}
                \label{fig:rsa_violins_4}
    \end{figure}

    \begin{figure}
        \includegraphics[width=\linewidth]{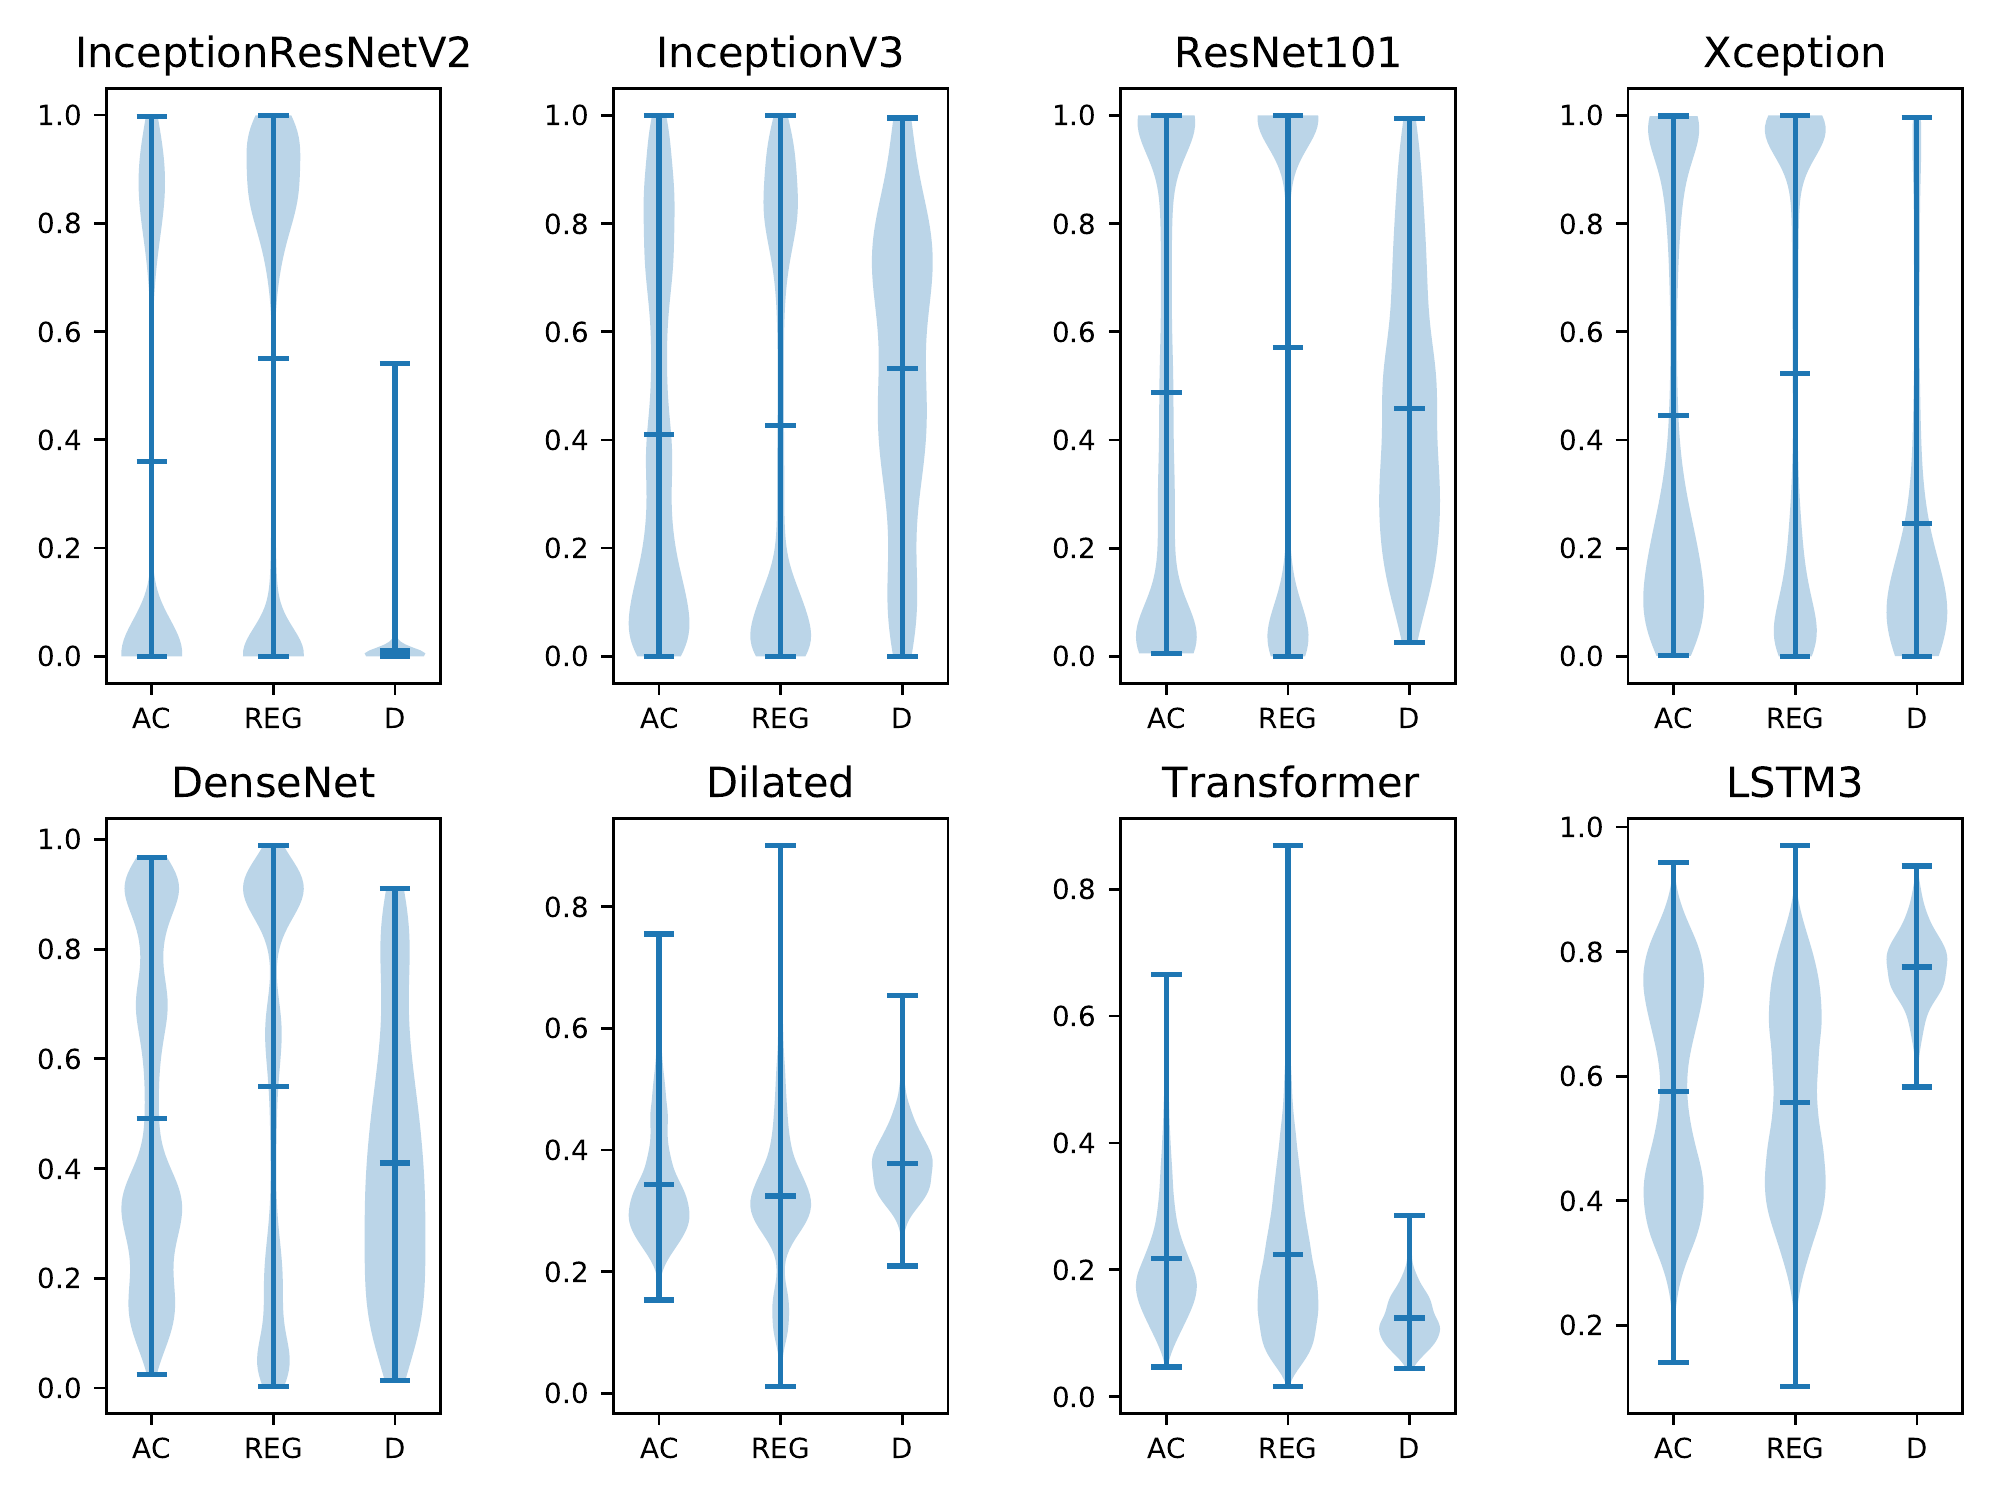}
        %   \caption{Another representation of the L2 norm output in which each violin represents the dissimilarity in a particular grouping. "AC" stands for across, and is the dissimilarity across features (such as between asymmetric and symmetric images).}
          \label{fig:rsa_violins_5}
    \end{figure}

    \begin{figure}
        \includegraphics[width=\linewidth]{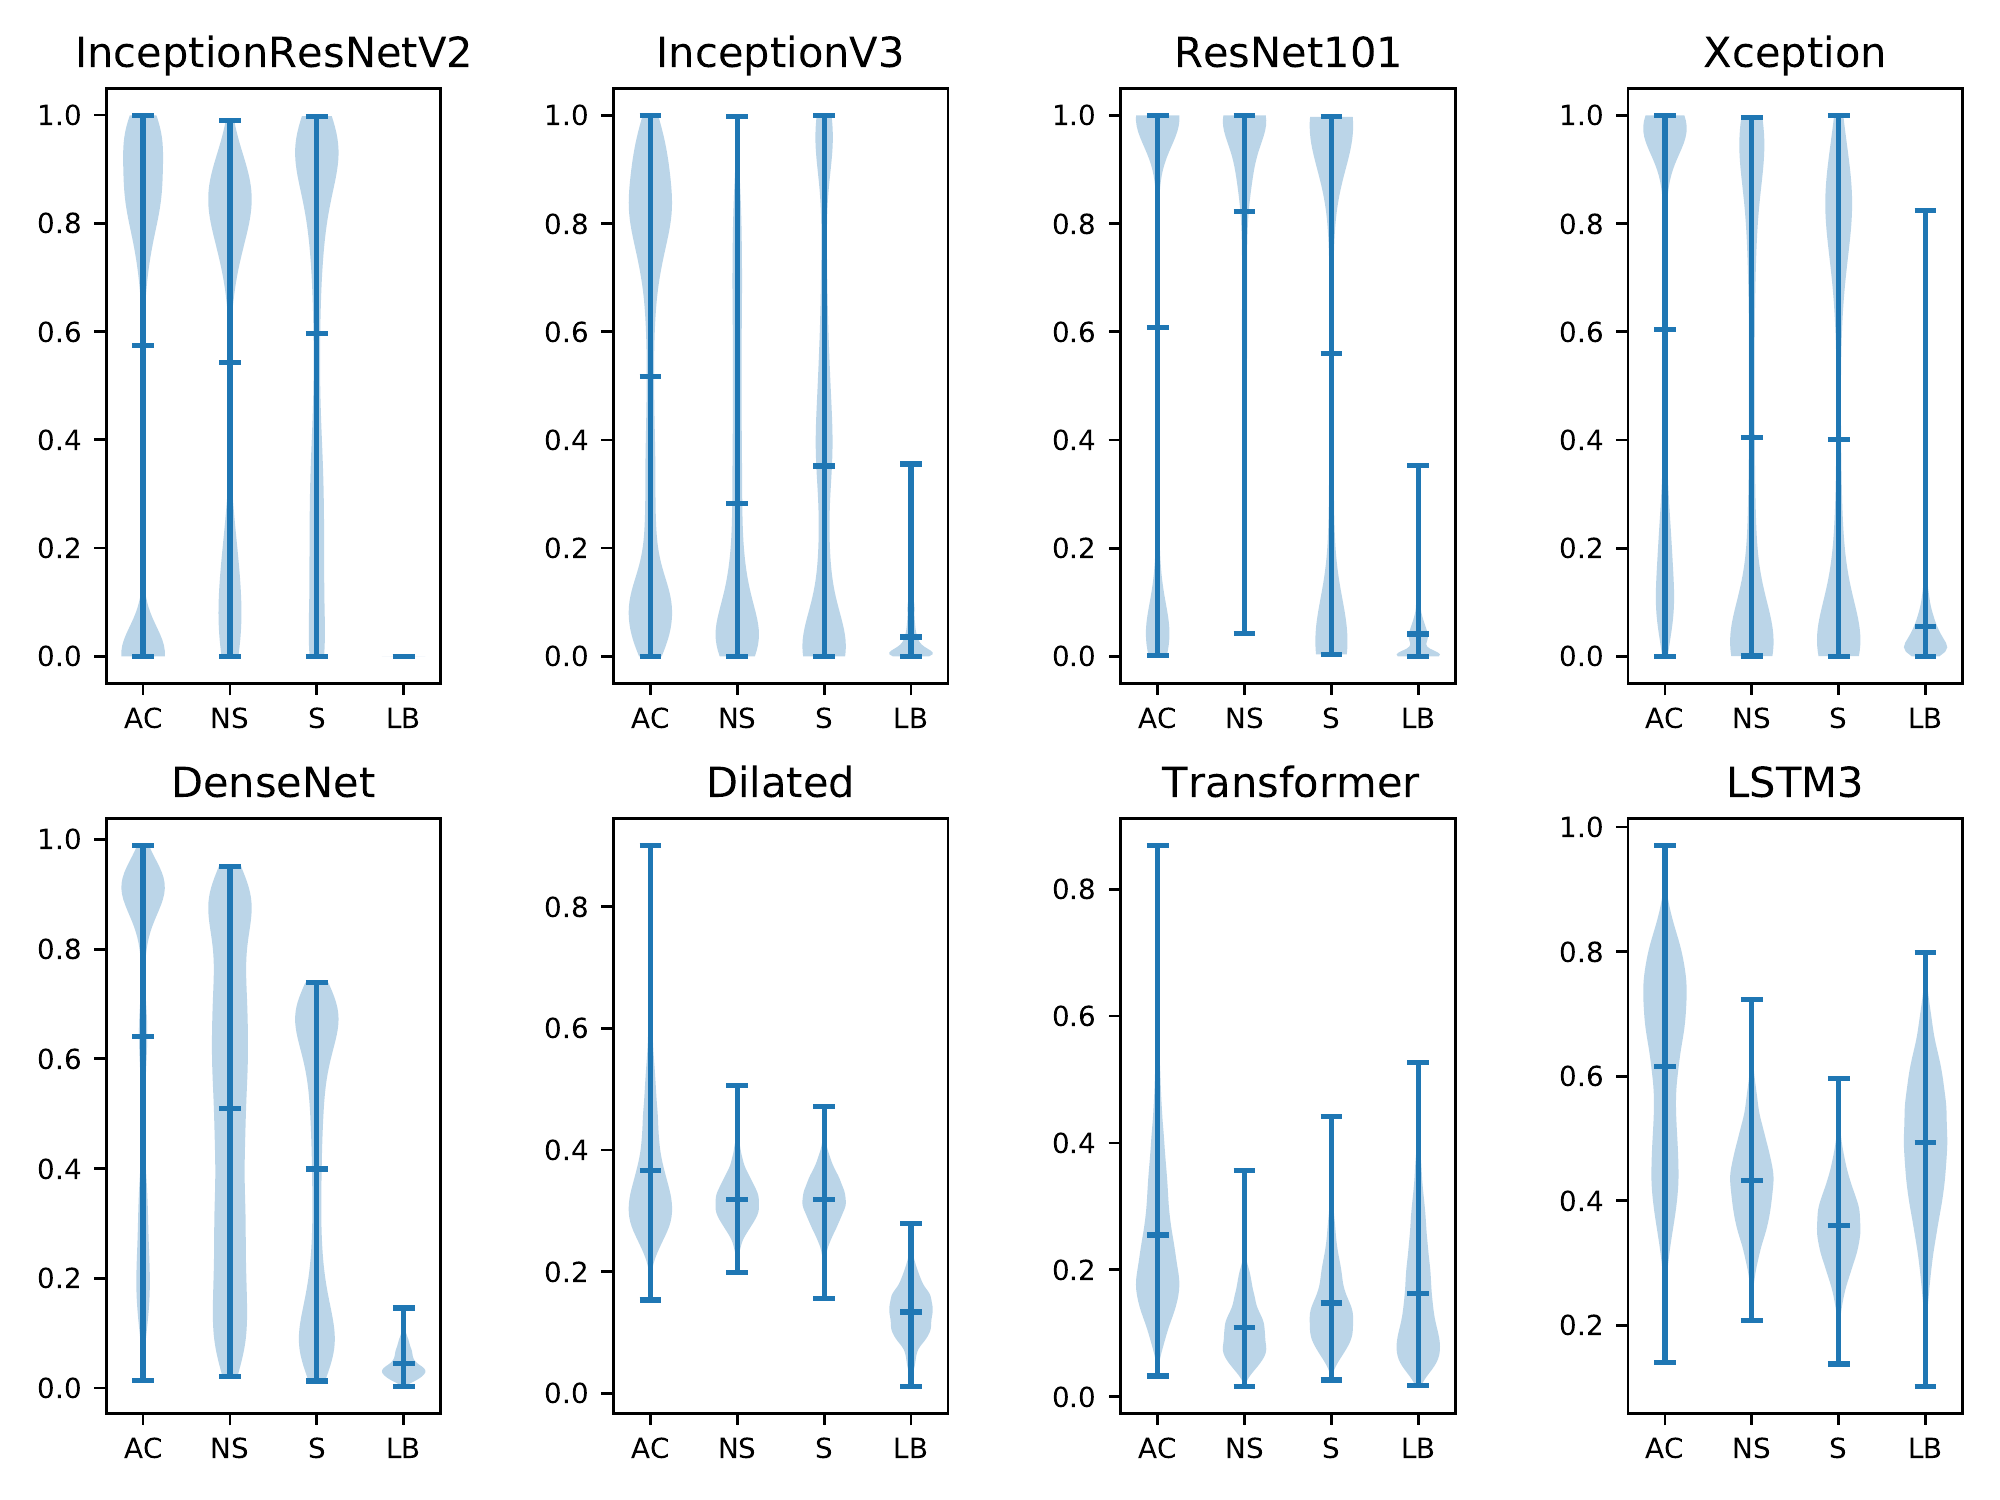}
        %   \caption{Another representation of the L2 norm output in which each violin represents the dissimilarity in a particular grouping. "AC" stands for across, and is the dissimilarity across features (such as between asymmetric and symmetric images).}
          \label{fig:rsa_violins_6}
    \end{figure}
